# Supplementary material for: An Optimized Construction of Lie Algebra Generator Pools for Variational Quantum Eigensolvers in Chemistry
Source: arXiv:2511.22593 ancillary file (2026-07-29)
Supplement: Supplementary file 1 [file MCPs-SI.pdf]

***Supplementary Materials:***  
*An Optimal Framework for Constructing Lie-Algebra Generator Pools:*  
*Application to Variational Quantum Eigensolvers for Chemistry*

Yaromir Viswanathan, Olivier Adjoua, César Féniau, Siwar Badreddine\*, Jean-Philip Piquemal\*

siwar.badreddine@qubit-pharmaceuticals.com,  
jean-philip.piquemal@sorbonne-universite.fr

November 27, 2025

## 1 Preliminaries

### 1.1 Proposition on Commutators

**Proposition 1.1.** (*Commutators*) Let  $P_1, P_2 \in i\mathcal{P}_N^*$ , we have

$$[P_1, P_2] = \begin{cases} 0, \\ 2P_1P_2 = \pm 2P_3, \quad P_3 \in i\mathcal{P}_N^*. \end{cases} \quad (1)$$

Therefore, the Pauli strings can only either commute or anti-commute.

*Proof.* Consider  $\alpha = iP_\alpha = i(\alpha_1 \otimes \cdots \otimes \alpha_N)$  and  $\beta = iP_\beta = i(\beta_1 \otimes \cdots \otimes \beta_N)$  where  $\alpha_i, \beta_i \in \{I, X, Y, Z\}$ , then

$$\begin{aligned} [\alpha, \beta] &= \alpha\beta - \beta\alpha = (-1)P_\alpha P_\beta + P_\beta P_\alpha \\ &= (\beta_1\alpha_1 \otimes \cdots \otimes \beta_n\alpha_n) - (\alpha_1\beta_1 \otimes \cdots \otimes \alpha_n\beta_n) \\ &= (\beta_1\alpha_1 \otimes \cdots \otimes \beta_n\alpha_n) + (-1)^\lambda (\beta_1\alpha_1 \otimes \cdots \otimes \beta_n\alpha_n), \end{aligned}$$

where  $\lambda$  is the total number of anti-commuting pairs  $(\alpha_i, \beta_i)$ , such that  $\alpha_i\beta_i = -\beta_i\alpha_i$ . Hence, either  $[\alpha, \beta] = 2\alpha\beta$  or  $[\alpha, \beta] = 0$ . Let's explore the case where  $[\alpha, \beta] = 2\alpha\beta$ . Assuming this, we have that

$$[\alpha, \beta] = 2(\beta_1\alpha_1 \otimes \cdots \otimes \beta_n\alpha_n).$$

Now, note that at least  $\beta_i\alpha_i$  term is not equal to the identity, and is equal to  $\pm i\sigma$ , where  $\sigma$  is a Pauli string, hence

$$[\alpha, \beta] = (-1)^{\lambda'} 2i(\sigma_1 \otimes \cdots \otimes \sigma_n),$$

where  $\sigma_i \in \{I, X, Y, Z\}$  and  $\lambda'$  counts the number of times a  $\beta_i\alpha_i$  term produces a  $-\sigma_i$  term. Hence,  $[\alpha, \beta]$  is indeed of the form  $\pm 2P$ , where  $P \in i\mathcal{P}_N^*$ .  $\square$

## 2 Main theorems

In this section, we provide a step-by-step proof for Theorem 2.1, which establishes the MCP congruence relation as follows

**Theorem 2.1.** (*MCP Congruence Theorem*) *A bracket-independent set of Pauli strings  $\mathcal{A}$  is an MCP for a given Lie algebra  $\mathfrak{g}$  if and only if there exists an invertible matrix  $\mathbf{P} \in \mathcal{M}_{|\mathcal{A}| \times |\mathcal{A}|}(\mathbb{F}_2)$  such that*

$$\mathbf{P}^\top \mathbf{\Gamma}_{\mathcal{A}} \mathbf{P} = \mathbf{\Gamma}_{\text{canonical, MCP}},$$

where  $\mathbf{\Gamma}_{\text{canonical, MCP}}$  is a canonical binary matrix for an MCP of  $\mathfrak{g}$ . Equivalently,

$$\mathbf{\Gamma}_{\mathcal{A}} \sim \mathbf{\Gamma}_{\text{canonical, MCP}},$$

where  $\sim$  denotes the congruence relation for matrices in  $\mathcal{M}_{|\mathcal{A}| \times |\mathcal{A}|}(\mathbb{F}_2)$ .

The following proof is based on the properties of the anti-commutation graphs defined in [1]. To proceed, we must first define a *contraction* operation applicable to the  $\mathbf{\Gamma}_{\mathcal{A}}$  matrices (the adjacency matrices of these graphs). The core of the proof is to show that for a given set of Pauli strings, its  $\mathbf{\Gamma}_{\mathcal{A}}$  matrix can be transformed via a sequence of these contractions into a final  $\mathbf{\Gamma}_{\text{equiv}}$  matrix, which we can identify as belonging to a known MCP.

**Definition 2.2.** *A contraction of  $\alpha$  by  $\beta$  is defined as*

$$\begin{aligned} c_\beta : i\mathcal{P}_N^* &\longrightarrow i\mathcal{P}_N^* \\ \alpha &\longmapsto \frac{1}{2}[\alpha, \beta]. \end{aligned}$$

For our purposes, we will always assume that all contractions happen between two anti-commuting Pauli strings, and hence  $\frac{1}{2}[\alpha, \beta] = \alpha\beta$ . The factor of  $\frac{1}{2}$  is introduced to make sure that  $i\mathcal{P}_N^*$  is closed under contractions.

**Proposition 2.3.** *Given a set  $\mathcal{A}$ , if we contract one of the elements by another (assuming that they anti-commute), we do not change the bracket closure  $\langle \mathcal{A} \rangle_{[.,.]}$  of  $\mathcal{A}$ .*

*Proof.* Let  $\alpha, \beta \in \mathcal{A}$  be anti-commuting elements. When we contract  $\alpha$  by  $\beta$ , we replace  $\alpha$  in  $\mathcal{A}$  by  $\alpha' := \alpha\beta$ , creating a modified set  $\mathcal{A}' := (\mathcal{A} \setminus \{\alpha\}) \cup \{\alpha'\}$ . We want to show that  $\langle \mathcal{A} \rangle_{[.,.]} = \langle \mathcal{A}' \rangle_{[.,.]}$ . We have

$$c_\beta(\alpha) = \alpha' = \frac{1}{2}[\alpha, \beta] = \alpha\beta. \quad (2)$$

It follows:

$$[\alpha', \beta] = \alpha'\beta - \beta\alpha' = \alpha\beta\beta - \beta\alpha\beta = \alpha I - (-1)\beta\beta\alpha = \alpha I + I\alpha = 2\alpha, \quad (3)$$

where we used two properties: first, that Pauli strings are involutory (i.e.,  $\alpha^2 = I$  for any Pauli string  $\alpha$ ), and second, that  $\alpha$  and  $\beta$  anticommute (i.e.,  $\alpha\beta = -\beta\alpha$ ). Since we have shown that  $\alpha$  can generate  $\alpha'$ , and  $\alpha'$  can in turn generate  $\alpha$  via the adjoint of  $\beta$ , we conclude that both bracket closures are equal.  $\square$

An interesting property is observed above and described in the following Lemma

**Lemma 2.4.** *Let  $\alpha, \beta \in i\mathcal{P}_N^*$  be anti-commuting elements. The contraction of  $\alpha$  by  $\beta$  gives  $\alpha' := \alpha\beta$  and the contraction of  $\alpha'$  by  $\beta$  gives  $c_\beta(\alpha') = \frac{1}{2}[\alpha', \beta] = \alpha$ . This shows that contraction maps are involutions (we keep, of course, the assumption that  $\alpha, \beta$  anticommute).*

We recall the definition of  $\Gamma_{\mathcal{A}}$  as the adjacency matrix of the anti-commutation graph introduced in [1]

**Definition 2.5.** *Given a set of Pauli strings  $\mathcal{A} := \{P_i\}_{i \in [|\mathcal{A}|]}$ , we define  $\Gamma_{\mathcal{A}} \in \mathcal{M}_{|\mathcal{A}| \times |\mathcal{A}|}(\mathbb{F}_2)$  as the binary matrix*

$$\Gamma_{\mathcal{A}}(i, j) := \begin{cases} 0, & [P_i, P_j] = 0, \\ 1, & \text{else.} \end{cases}$$

*This matrix contains all commutation relations between elements in  $\mathcal{A}$ . Note that  $\Gamma_{\mathcal{A}}$  matrices always have zero diagonal entries and are symmetric.*

For simplicity, we work in  $\mathbb{F}_2^{2N}$  and use some ideas from [8]. For starter, we define the Pauli group  $\mathcal{G}_{\mathcal{P}_N}$

**Definition 2.6.** *(Pauli Group [8]) Recall the set of Pauli strings  $\mathcal{P}_N := \{I, X, Y, Z\}^{\otimes N}$ . The Pauli group (on  $N$  qubits) is the set generated by  $\mathcal{P}_N$  via matrix multiplication as the group operation, i.e.,*

$$\mathcal{G}_{\mathcal{P}_N} := \langle \mathcal{P}_N \rangle.$$

*Using well-known properties of products of Pauli strings, we have a more explicit formulation via*

$$\mathcal{G}_{\mathcal{P}_N} = \{\lambda P \mid P \in \mathcal{P}_N, \lambda \in \{\pm 1, \pm i\}\}.$$

**Definition 2.7.** *([8]) Recall that  $Y = iXZ$ , hence, it is possible to write any  $\lambda P \in \mathcal{G}_{\mathcal{P}_N}$  as*

$$\lambda P = \lambda' P_X P_Z.$$

*Note that  $P = \alpha_1 \otimes \cdots \otimes \alpha_n$ ,  $\alpha_i \in \{I, X, Y, Z\}$ , so we have that  $P_X = \beta_1 \otimes \cdots \otimes \beta_n$ ,  $\beta_i \in \{I, X\}$  with  $\beta_i = X$  only if  $\alpha_i = X$  or  $\alpha_i = Y$  (and  $\beta_i = I$ , otherwise), and similarly, we have that  $P_Z = \gamma_1 \otimes \cdots \otimes \gamma_n$ ,  $\gamma_i \in \{I, Z\}$  with  $\gamma_i = Z$  only if  $\alpha_i = Z$  or  $\alpha_i = Y$ . Note that since  $XZ = -iY$ , we have to multiply by a factor of  $i$  to recover  $Y$  each time  $P_X$  and  $P_Z$  have a non-identity term, hence, we have that  $\lambda' = \lambda \cdot (n_y i)$ , where  $n_y$  is the number of times that  $Y$  appears in the Pauli string forming  $P$ . Writing an element in the Pauli group as  $\lambda P_X P_Z$  is known as writing it in standard form.*

**Definition 2.8.** *([8]) Let  $\mathcal{S} \subseteq \mathcal{P}_N$  be a subgroup of  $\mathcal{G}_{\mathcal{P}_N}$  with the following properties:*

- $\mathcal{S}$  is closed under multiplication in  $\mathcal{G}_{\mathcal{P}_N}$ , i.e., is a subgroup of the Pauli group.
- $[\mathcal{S}, \mathcal{S}] = \{0\}$ .
- $-I \notin \mathcal{S}$

Now we introduce the operator  $\phi$  acting on  $\mathcal{S}$

**Proposition 2.9.** *We write a standard form as  $\lambda P_X P_Z = \lambda(\alpha_1 \otimes \cdots \otimes \alpha_n)(\beta_1 \otimes \cdots \otimes \beta_n)$ . Consider the function*

$$\begin{aligned} \phi : \mathcal{S} &\longrightarrow \mathbb{F}_2^{2N} \\ \lambda P_X P_Z &\mapsto v, \end{aligned}$$

where  $v$  is given by the following

$$v[i] := \begin{cases} 1, & \alpha_i = X \\ 0, & \alpha_i = I \end{cases}$$

$$v[N+i] := \begin{cases} 1, & \beta_i = Z \\ 0, & \beta_i = I, \end{cases}$$

where  $v[i]$  (resp.  $v[N+i]$ ) refers to the entry of  $v$  at index  $i$  (resp.  $N+i$ ). We claim that this function is a group isomorphism between  $\mathcal{S}$  and  $\mathbb{F}_2^{2N}$ , where the latter is considered an additive group.

*Proof.* Immediately, one might worry about the  $\lambda$  term and think that  $\phi$  is not even injective as  $\pm P_X P_Z, \pm i P_X P_Z$  would all get mapped to the same  $v$ , however, recall that  $\mathcal{S}$  is a subset of  $\mathcal{P}_N$ , not  $\mathcal{G}_{\mathcal{P}_N}$ , so in other words, only one of the scaling factors in  $\{\pm 1, \pm i\}$  will correct the term  $P_X P_Z$  to be a valid Pauli string by balancing out the  $i$  factors created as a byproduct of the  $XZ$  terms. Otherwise, by construction, it is obvious that this function is a bijection. Let  $P = \lambda P_X P_Z$  and let  $Q = \lambda' P'_X P'_Z$ , we have

$$\phi(P) = (a_1, \dots, a_N, b_1, \dots, b_N), a_i, b_i \in \{0, 1\},$$

and

$$\phi(Q) = (c_1, \dots, c_N, d_1, \dots, d_N), c_i, d_i \in \{0, 1\},$$

we have

$$\phi(P) + \phi(Q) = (a_1 \oplus c_1, \dots, a_N \oplus c_N, b_1 \oplus d_1, \dots, b_N \oplus d_N), \quad (4)$$

where  $a_i \oplus c_i = a_i + c_i \pmod{2}, i \in [N]$ . We also have

$$PQ = \lambda \lambda' P_X P_Z P'_X P'_Z = (-1)^\gamma \lambda \lambda' (P_X P'_X)(P_Z P'_Z),$$

where  $\gamma$  is defined as the parity of the number of tensor product slots where both an  $X$  appears in  $P'_X$  and a  $Z$  appears in  $P_Z$ . Now let  $\phi(P \circ Q) = v$ , we have that for  $i \in [N]$

$$v[i] = a_i \oplus c_i, \quad (5)$$

and similarly for the second half of the vector:

$$v[N+i] = b_i \oplus d_i. \quad (6)$$

Therefore, we conclude that the map  $\phi$  is a homomorphism:

$$\phi(P \circ Q) = \phi(P) \oplus \phi(Q). \quad (7)$$

Note that the  $(-1)^\gamma \lambda \lambda'$  is of no importance since only one such scaling factor produces a valid Pauli string.  $\square$

**Proposition 2.10.**  $\phi$  is a group isomorphism, if some  $\alpha \in \mathcal{S}$  can be decomposed as  $\alpha = \beta_1 \circ \dots \circ \beta_n; \beta_i \in \mathcal{S} \setminus \{\alpha\}$ , it immediately follows that

$$\phi(\alpha) = \phi(\beta_1 \circ \dots \circ \beta_n) = \phi(\beta_1) + \dots + \phi(\beta_n).$$

Hence, we have that the "product-independence" of  $\mathcal{S}$  (i.e., no one element in  $\mathcal{S}$  can be written as some product of the others), is equivalent to the linear independence of  $\phi(\mathcal{S})$  in  $\mathbb{F}_2^{2N}$ .

Since we have already translated the notion of *product-independence* into *linear independence* via  $\phi$ , maybe we can do the same for the commutativity relation. Let us consider the following proposition

**Proposition 2.11.** ([8]) Let  $\Lambda$  be defined as

$$\Lambda := \begin{pmatrix} 0_N & I_N \\ I_N & 0_N \end{pmatrix} \in \mathbb{F}_2^{2N \times 2N}.$$

For any pair  $\alpha, \beta \in \mathcal{G}_{\mathcal{P}_N}$ , we have:

$$[\alpha, \beta] = 0 \in \mathbb{C}^N \iff \phi(\alpha)^\top \Lambda \phi(\beta) = 0 \in \mathbb{F}_2.$$

*Proof.* We write  $\alpha = P_X P_Z$  and  $\beta = P'_X P'_Z$  and forget about the scaling factors, because they always commute, anyway. Additionally, let us denote  $\phi(\alpha)$  as  $(v_X^\alpha, v_Z^\alpha)^\top$  and  $\phi(\beta)$  as  $(v_X^\beta, v_Z^\beta)^\top$ , where  $v_X^\alpha$  is the first half of the array representing  $\phi(\alpha)$  which pertains only to the  $P_X$  part in  $\alpha$ 's standard form in  $\mathcal{G}_{\mathcal{P}_N}$ , and similarly for  $v_Z^\alpha, v_X^\beta, v_Z^\beta$ . Note the following

$$\begin{aligned} \Lambda \phi(\beta) &= (v_Z^\beta, v_X^\beta)^\top \\ \phi(\alpha)^\top \Lambda \phi(\beta) &= (v_X^\alpha, v_Z^\alpha)(v_Z^\beta, v_X^\beta)^\top = m \oplus n, \end{aligned}$$

where  $m$  is the number of times where an  $X$  appears in  $P_X$  in the same tensor product slot as a  $Z$  in  $P'_Z$  and  $n$  is the same thing but with a  $Z$  in the same slot as an  $X$  in  $P_Z$  and  $P'_X$ , respectively. Now let us try to understand the condition that assures  $\alpha, \beta$  commute

$$\begin{aligned} \alpha\beta &= (P_X P_Z)(P'_X P'_Z) \\ &= (-1)^\lambda (P_X P'_X)(P_Z P'_Z) \\ &= (-1)^\lambda (P'_X P_X)(P'_Z P_Z) \\ &= (-1)^{\lambda+\mu} (P'_X P'_Z)(P_X P_Z), \end{aligned}$$

where  $\mu$  is similar to  $\lambda$  and is defined as the parity of the number of tensor product slots where both an  $X$  appears in  $P_X$  and a  $Z$  appears in  $P'_Z$ . We can conclude that  $\mu = m$ . Clearly, we have that  $\alpha, \beta$  commute when  $\lambda \oplus \mu = 0$ , which is indeed equivalent to  $\phi(\alpha)^\top \Lambda \phi(\beta) \cong 0 \pmod{2}$ .  $\square$

**Remark 2.12.** Recall that since  $i\mathcal{P}_N^*$  contains all Pauli strings (multiplied by  $i$ ) except for the identity, we have that  $\phi(i\mathcal{P}_N^*) = \mathbb{F}_2^{2N} \setminus \{0\}$ .

We can now define the contraction operation in  $\mathbb{F}_2^{2N}$ :

**Proposition 2.13.** In the context of  $\mathbb{F}_2^{2N}$ , a contraction of  $\alpha \in i\mathcal{P}_N^*$  by  $\beta \in i\mathcal{P}_N^*$  corresponds to replacing  $\phi(\alpha)$  by  $\phi(\alpha\beta) = \phi(\alpha) + \phi(\beta)$ .

**Definition 2.14.** We introduce the following notation  $\langle \alpha, \beta \rangle_\Lambda := \alpha^\top \Lambda \beta$ , for  $\alpha, \beta \in \mathbb{F}_2^{2N}$ .

Now we can redefine  $\Gamma_{\mathcal{A}}$  matrices using our previous definitions instead of relying directly on the anti-commutation graph

**Definition 2.15.** Consider a set  $\phi(\mathcal{A}) := \{\tilde{\alpha}_1, \dots, \tilde{\alpha}_n\} \subseteq \mathbb{F}_2^{2N}$ , we will define the matrix  $\Gamma_{\mathcal{A}}$  by

$$\Gamma_{\mathcal{A}} := \begin{pmatrix} \langle \tilde{\alpha}_1, \tilde{\alpha}_1 \rangle_\Lambda & \cdots & \langle \tilde{\alpha}_1, \tilde{\alpha}_n \rangle_\Lambda \\ \langle \tilde{\alpha}_2, \tilde{\alpha}_1 \rangle_\Lambda & \cdots & \langle \tilde{\alpha}_2, \tilde{\alpha}_n \rangle_\Lambda \\ \vdots & \vdots & \vdots \\ \langle \tilde{\alpha}_n, \tilde{\alpha}_1 \rangle_\Lambda & \cdots & \langle \tilde{\alpha}_n, \tilde{\alpha}_n \rangle_\Lambda \end{pmatrix}.$$

Note that this matrix is clearly symmetric as  $\langle \tilde{\alpha}_i, \tilde{\alpha}_j \rangle_\Lambda = \langle \tilde{\alpha}_j, \tilde{\alpha}_i \rangle_\Lambda$  and has a main diagonal of 0s.

The following example illustrates the connection between  $\Gamma_{\mathcal{A}}$  matrices and changes in the anti-commutation graph.

**Example 2.16.** We start with this set  $\phi(\mathcal{A}) := \{\alpha_1, \alpha_2, \alpha_3, \alpha_4, \alpha_5\}$  where

$$\alpha_1 := \begin{pmatrix} 1 \\ 0 \\ 0 \\ 0 \end{pmatrix}, \alpha_2 := \begin{pmatrix} 0 \\ 1 \\ 0 \\ 0 \end{pmatrix}, \alpha_3 := \begin{pmatrix} 0 \\ 0 \\ 1 \\ 0 \end{pmatrix}, \alpha_4 := \begin{pmatrix} 0 \\ 0 \\ 0 \\ 1 \end{pmatrix}$$

and  $\alpha_5 = \alpha_1 + \alpha_3$ . Next, we compute the  $\Gamma_{\mathcal{A}}$  matrix, obtaining

$$\Gamma_{\mathcal{A}} = \begin{pmatrix} 0 & 1 & 1 & 0 & 1 \\ 1 & 0 & 1 & 0 & 0 \\ 1 & 1 & 0 & 1 & 1 \\ 0 & 0 & 1 & 0 & 1 \\ 1 & 0 & 1 & 1 & 0 \end{pmatrix}.$$

Using the  $\Gamma_{\mathcal{A}}$  matrix, we can draw the following anti-commuting graph

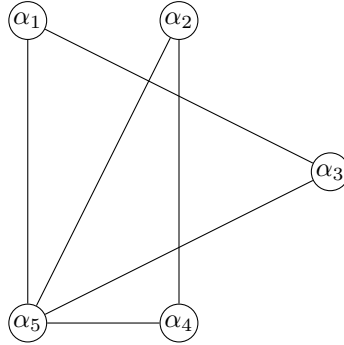

Now, consider the contraction of  $\alpha_1$ , by  $\alpha_3$  (note that they anticommute). The node  $\alpha_1$  now becomes  $\alpha_1 + \alpha_3$ , so our new set is  $\mathcal{A}' := \{\alpha'_1 := \alpha_1 + \alpha_3, \alpha_2, \alpha_3, \alpha_4, \alpha_5\}$ . For now, assume we just blindly recompute the new  $\Gamma_{\mathcal{A}'}$  matrix. Doing this yields the following new  $\Gamma_{\mathcal{A}'}$  matrix and graph

$$\Gamma_{\mathcal{A}'} = \begin{pmatrix} 0 & 0 & 1 & 0 & 0 \\ 0 & 0 & 0 & 1 & 1 \\ 1 & 0 & 0 & 0 & 1 \\ 0 & 1 & 0 & 0 & 1 \\ 0 & 1 & 1 & 1 & 0 \end{pmatrix},$$

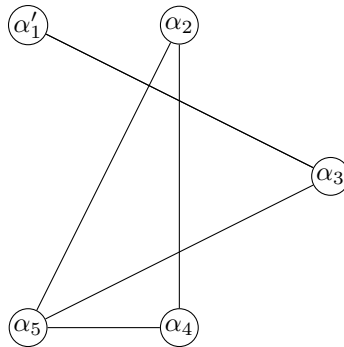

Notice how this contraction disconnected the first node from the fifth node. Despite this, the bracket closure of this set remains the same according to Proposition 2.3

The central idea is that a sequence of such contractions can reduce the graph to a canonical form. This transformation corresponds to finding a matrix equivalent to the original  $\mathbf{\Gamma}_{\mathcal{A}}$ . We now state the following proposition

**Proposition 2.17.** *A contraction is equivalent to applying elementary row operations (EROs) on  $\mathbf{\Gamma}_{\mathcal{A}}$ .*

*Proof.* Assume that we take a given node  $\alpha_i$  and contract it by  $\alpha_j$ , thus replacing  $\alpha_i$  in the set by  $\alpha_i + \alpha_j$ , then, we note the following

$$\begin{aligned}\langle \alpha_k, \alpha_i + \alpha_j \rangle_{\Lambda} &= \langle \alpha_k, \alpha_i \rangle_{\Lambda} + \langle \alpha_k, \alpha_j \rangle_{\Lambda} \\ &= \langle \alpha_i + \alpha_j, \alpha_k \rangle_{\Lambda} = \langle \alpha_i, \alpha_k \rangle_{\Lambda} + \langle \alpha_j, \alpha_k \rangle_{\Lambda}.\end{aligned}$$

Note that the  $i$ -th column of the  $\mathbf{\Gamma}_{\mathcal{A}}$  matrix contains  $\langle \alpha_k, \alpha_i \rangle$  and the  $i$ -th row contains  $\langle \alpha_i, \alpha_k \rangle$ , hence, when we contract and replace  $\alpha_i$  by  $\alpha_i + \alpha_j$ , all we need to do to find the new  $\mathbf{\Gamma}_{\mathcal{A}'}$  matrix is simply, first, add the  $j$ -th row of  $\mathbf{\Gamma}_{\mathcal{A}}$  to the  $i$ -th row of  $\mathbf{\Gamma}_{\mathcal{A}}$ , creating intermediate matrix  $\mathbf{\Gamma}$ , and secondly add the  $j$ -th column of  $\mathbf{\Gamma}_{\mathcal{A}}$  - **not**  $\mathbf{\Gamma}$  - to the  $i$ -th column of  $\mathbf{\Gamma}$ , creating  $\mathbf{\Gamma}_{\mathcal{A}'}$ . Note that operation of additions may be reversed as long as we keep in mind that the first operation (either row sum or column sum) will create a  $\mathbf{\Gamma}$  matrix, and that the second operation will add a row or column from  $\mathbf{\Gamma}_{\mathcal{A}}$  to  $\mathbf{\Gamma}$ .  $\square$

**Proposition 2.18.** *Let  $\mathcal{A}$  be a set of Pauli strings. There exists an invertible matrix  $\mathbf{P} \in \mathcal{M}_{|A| \times |A|}(\mathbb{F}_2)$  such that*

$$\mathbf{P}^{\top} \mathbf{\Gamma}_{\mathcal{A}} \mathbf{P} = \mathbf{\Gamma}_{equiv},$$

*equivalently,*

$$\mathbf{\Gamma}_{\mathcal{A}} \sim \mathbf{\Gamma}_{equiv},$$

*where  $\sim$  denotes the congruence relation for matrices in  $\mathcal{M}_{|A| \times |A|}(\mathbb{F}_2)$ .*

*Proof.* Consider a given  $\mathbf{\Gamma}_{\mathcal{A}}$  matrix corresponding to a set  $\mathcal{A} := \{\alpha_i\}_{i \in [|A|]}$ . When we contract  $\alpha_i$  by  $\alpha_j$ , we replace  $\alpha_i$  by  $\alpha_i + \alpha_j$ . Let us assume we always start with the row sum. Then, the intermediate matrix  $\mathbf{\Gamma}$  is obtained by

$$\mathbf{\Gamma} = \begin{pmatrix} e_1^{\top} \\ \vdots \\ (e_i + e_j)^{\top} \\ \vdots \\ e_{|A|}^{\top} \end{pmatrix} \mathbf{\Gamma}_{\mathcal{A}},$$

where  $(e_i + e_j)^{\top}$  is the  $i$ -th row of the ERO matrix on the left. Note that this operation affects the  $(i, i)$ -th entry, and hence, changes the  $i$ -th column, which is what we need to handle next. However, note that the  $(i, i)$ -th entry must always be 0, however, since  $\mathbf{\Gamma}_{\mathcal{A}}$  is symmetric and  $\alpha_i, \alpha_j$  anticommute, the  $(i, i)$ -th entry of  $\mathbf{\Gamma}$  will always be a 1. This entry will be set back to 0 when we proceed with the next operation involving columns, so this isn't an issue. However, this operation also changes the  $(j, i)$ -th entry of the  $\mathbf{\Gamma}_{\mathcal{A}}$  matrix. This is exactly why we can't just blindly add the  $j$ -th column of  $\mathbf{\Gamma}$  to the  $i$ -th column of  $\mathbf{\Gamma}$ . However this operation turns the  $(i, j)$ -th of  $\mathbf{\Gamma}$  into  $\langle \alpha_i, \alpha_j \rangle_{\Lambda}$ . Therefore, the  $j$ -th column of  $\mathbf{\Gamma}_{\mathcal{A}}$  and  $\mathbf{\Gamma}$  are actually the same.

It follows that we can actually blindly proceed by adding the  $j$ -th column of  $\mathbf{\Gamma}$  to the  $i$ -th column of  $\mathbf{\Gamma}$ . Once again, recall that we could have swapped the order of operations (either

adding the row first, or the column first), which thankfully, coincides with the associativity of matrix multiplication. Now that we have  $\mathbf{\Gamma}$ , we need to do the column operation. We have that

$$\mathbf{\Gamma}_{\mathcal{A}'} = \mathbf{\Gamma} \begin{pmatrix} e_1 & \cdots & (e_i + e_j) & \cdots & e_{|\mathcal{A}|} \end{pmatrix},$$

where  $e_i + e_j$  is the  $i$ -th column of the ERO matrix on the right. Note that this ERO matrix on the right is actually the transpose of the ERO matrix on the left that transformed  $\mathbf{\Gamma}_{\mathcal{A}}$  into  $\mathbf{\Gamma}$  in the previous step. This operation fixes the earlier problem of the  $(i, i)$ -th entry being 1, it is now set back to 0. Let us write this two-step process as

$$\mathbf{\Gamma}_{\mathcal{A}'} = \rho_{i,j}^\top \mathbf{\Gamma} \rho_{i,j},$$

where  $\rho_{i,j}$  represents the ERO resulting from the contraction of  $\alpha_i$  by  $\alpha_j$ . It is worth noting that since we are working in  $\mathbb{F}_2$ , we have

$$\rho_{i,j} \rho_{i,j} = I,$$

such that the  $\rho_{i,j}$  ERO matrices are involutions. Ineed, the  $\rho_{i,j}$  matrices represent the action of the contraction of  $\alpha_i$  by  $\alpha_j$  on the level of the entire  $\mathbf{\Gamma}_{\mathcal{A}}$  matrix, and this involuntary property is retained at the level of the  $\mathbf{\Gamma}_{\mathcal{A}}$  matrix as well. If we denote the action of the contraction of  $\alpha_i$  by  $\alpha_j$  at the level of the  $\mathbf{\Gamma}_{\mathcal{A}}$  matrix as  $c_{i,j}^{\mathbf{\Gamma}_{\mathcal{A}}}$  where

$$c_{i,j}^{\mathbf{\Gamma}_{\mathcal{A}}}(\mathbf{\Gamma}_{\mathcal{A}}) := \rho_{i,j} \mathbf{\Gamma}_{\mathcal{A}} \rho_{i,j}^\top.$$

Then, we obtain

$$\begin{aligned} c_{i,j}^{\mathbf{\Gamma}_{\mathcal{A}}} \circ c_{i,j}^{\mathbf{\Gamma}_{\mathcal{A}}}(\mathbf{\Gamma}_{\mathcal{A}}) &= \rho_{i,j} (\rho_{i,j} \mathbf{\Gamma}_{\mathcal{A}} \rho_{i,j}^\top) \rho_{i,j}^\top \\ &= I \mathbf{\Gamma}_{\mathcal{A}} (\rho_{i,j} \rho_{i,j})^\top \\ &= I \mathbf{\Gamma}_{\mathcal{A}} I^\top \\ &= \mathbf{\Gamma}_{\mathcal{A}}. \end{aligned}$$

It follows, that for a given  $\mathbf{\Gamma}_{\mathcal{A}}$ , one can find sequence of contractions  $\rho_1, \dots, \rho_n$  that transform  $\mathbf{\Gamma}_{\mathcal{A}}$  into some  $\mathbf{\Gamma}_{\text{equiv}}$ . When we write this out fully as a composition of linear maps, we have

$$\mathbf{\Gamma}_{\text{equiv}} = \rho_n^\top \cdots \rho_1^\top \mathbf{\Gamma}_{\mathcal{A}} \rho_1 \cdots \rho_n,$$

which can be rewritten as

$$\mathbf{\Gamma}_{\text{equiv}} = (\rho_n \cdots \rho_1)^\top \mathbf{\Gamma}_{\mathcal{A}} (\rho_n \cdots \rho_1).$$

Hence, defining  $\mathbf{P} := \rho_n \cdots \rho_1$ , we have that

$$\mathbf{\Gamma}_{\text{equiv}} = \mathbf{P}^\top \mathbf{\Gamma}_{\mathcal{A}} \mathbf{P}.$$

The matrix  $\mathbf{P}$  is invertible which follows immediately from the fact that it is equal to a sequence of ERO matrices.  $\square$

So far, we have shown that for any set  $\mathcal{A}$  of Pauli strings and its associated matrix  $\mathbf{\Gamma}_{\mathcal{A}}$ , one can always find either a series of contractions or, equivalently, an invertible matrix  $\mathbf{P}$  that transforms  $\mathbf{\Gamma}_{\mathcal{A}}$  into  $\mathbf{\Gamma}_{\text{equiv}}$ . More interestingly, we will now show that if  $\mathbf{\Gamma}_{\text{equiv}}$  corresponds to a set  $\mathcal{A}_{MCP}$  (which is known to be an MCP) and if  $\mathcal{A}$  is bracket-independent, then we can conclude that  $\mathcal{A}$  is also an MCP.

We recall the definition of bracket-independent set as follows

**Definition 2.19.** (*Bracket-independent set*) A set  $\mathcal{A}$  of Pauli strings is bracket-independent if no element in the set can be expressed as adjoint sequence of other elements. Formally, for each  $P_j \in \mathcal{A}, j \in [|\mathcal{A}|]$ , we have

$$P_j \notin \langle \mathcal{A} / \{P_j\} \rangle_{[.,.]}, \quad (8)$$

where  $\langle \mathcal{A} \rangle_{[.,.]} := \bigcup_{n \in \mathbb{N}} \{ad_{\alpha_n} \circ \dots \circ ad_{\alpha_1}(\alpha_0) \in \mathfrak{g} \mid (\alpha_i)_{i \in [n]} \subseteq \mathcal{A}\}$ ,

where the adjoint endomorphism, denoted as  $ad_{\alpha_i}$ , is defined as

**Definition 2.20.** (*adjoint endomorphism*) The adjoint  $ad_{\alpha}$  of an element  $\alpha \in \mathfrak{g}$  is the endomorphism defined as

$$\begin{aligned} ad_{\alpha} : \mathfrak{g} &\mapsto \mathfrak{g} \\ \beta &\mapsto [\alpha, \beta] = \alpha\beta - \beta\alpha. \end{aligned} \quad (9)$$

Similarly we can write in  $\mathbb{F}_2^{2N}$ :

**Definition 2.21.** We define  $ad_{\alpha}$  for  $\alpha \in \mathbb{F}_2^{2N}$  as

$$\begin{aligned} ad_{\alpha} : \mathbb{F}_2^{2N} &\Longrightarrow \mathbb{F}_2^{2N} \\ \beta &\longmapsto (\alpha^{\top} \Lambda \beta)(\alpha + \beta). \end{aligned}$$

Recall that the scalar  $\alpha^{\top} \Lambda \beta = 0$  when  $\alpha, \beta$  commute and 1 when they anti commute.

**Definition 2.22.** For a set  $\mathcal{A} \subset \mathbb{F}_2^{2N}$ , we define it's "bracket closure" as

$$\langle \mathcal{A} \rangle_{[.,.]} := \bigcup_{n \in \mathbb{N}} \{ad_{\alpha_n} \dots ad_{\alpha_1}(\alpha_0) \mid \{\alpha_i\}_{i \in [n]} \in \mathcal{A}^n\},$$

which refers to the set of all possible "commutators" of elements in  $\mathcal{A}$ . This is completely analogous to subsets of  $i\mathcal{P}_N^*$ .

**Proposition 2.23.** Consider a basis  $\phi(\mathcal{A})$  for  $\mathbb{F}_2^{2N}$ , adding one vector to  $\mathcal{A}$  which is not bracket-independent w.r.t. the elements in  $\mathcal{A}$  will never yield an MCP.

*Proof.* For this proof, we proceed by a counter example, where we consider  $\mathfrak{g} := \mathfrak{su}(2^N)$ . It has been demonstrated in [8] that the minimum cardinality for an MCP is  $2N+1$ . However, according to Theorem 2 in [8], a basis for  $\mathbb{F}_2^{2N}$  will never generate all of  $\mathfrak{su}(2^N)$ , as it has cardinality  $2N$ . Consider  $\mathcal{A}' := \mathcal{A} \cup \{\alpha_{2N+1}\}$  where our new vector  $\alpha_{2N+1}$  is non-bracket-independent from the elements already in  $\mathcal{A}$ . Then

$$\langle \mathcal{A}' \rangle_{[.,.]} = \langle \mathcal{A} \rangle_{[.,.]}$$

This is clear from the fact that  $\alpha_{2N+1} \in \langle \mathcal{A} \rangle_{[.,.]}$  due to the assumption that  $\alpha_{2N+1}$  is not bracket-independent.  $\square$

**Remark 2.24.** Note that if we add a bracket-independent element  $\alpha_{2N+1}$  to  $\mathcal{A}$ , forming  $\mathcal{A}'$ , then, we will always have

$$\langle \mathcal{A} \rangle_{[.,.]} \subsetneq \langle \mathcal{A}' \rangle_{[.,.]}$$

This will indeed always be a proper subset, as witnessed by the new element  $\alpha_{2N+1} \notin \langle \mathcal{A} \rangle_{[.,.]}$  which is trivially in the bracket closure of  $\mathcal{A}'$ .

**Lemma 2.25.** Due to the proposition above, we can conclude that an MCP must be bracket-independent, i.e., no one element in the MCP can be written as an adjoint sequence of the other elements.

*Proof.* Note that for a basis in  $\mathbb{F}_2^{2N}$ , bracket-independence is implied by linear independence in  $\mathbb{F}_2^{2N}$ . This is because linear independence implies that no single element in  $\mathbb{F}_2^{2N}$  can be written as a sum of the others, and hence, can't be written as an adjoint sequence of the others. Hence, if we already assume the "best case" where  $\mathcal{A}$  is a basis, and hence, bracket-independent, then any set of cardinality  $2N$  can have a bracket closure with cardinality less than or equal to the bracket-closure's cardinality of  $\mathcal{A}$ . In other words, if we have a set  $\mathcal{B}$  which is bracket-dependent and of cardinality  $2N$ , then

$$|\langle \mathcal{B} \rangle_{[\cdot, \cdot]}| \leq |\langle \mathcal{A} \rangle_{[\cdot, \cdot]}| < |\mathfrak{su}(2^N)| \implies \langle \mathcal{B} \rangle_{[\cdot, \cdot]} \neq \mathfrak{su}(2^N).$$

Hence, we may conclude that an MCP must be bracket-independent.  $\square$

This leads us to Theorem 2.1, which states:

**Theorem 2.26.** *A bracket-independent set of Pauli strings  $\mathcal{A}$  is an MCP if and only if there exists an invertible matrix  $\mathbf{P} \in \mathbb{F}_2^{|A| \times |A|}$  such that*

$$\mathbf{P} \Gamma_{\mathcal{A}} \mathbf{P}^\top = \Gamma_{\text{canonical, MCP}},$$

where  $\Gamma_{\text{canonical, MCP}}$  is the canonical  $\Gamma$  matrix for MCPs (of a given dimension).

*Proof.* The proof follows immediately from the previous ideas and propositions.  $\square$

In what follows, we examine the properties of the  $\Gamma_{\mathcal{A}}$  matrices, which provides the basis for an efficient method to verify MCP sets. Inspired by the work of [4], the following matrix is introduced

**Definition 2.27.** ([4]) Define  $\mathbf{J}_N \in \mathcal{M}_{N \times N}(\mathbb{F}_2)$  as follows:

$$\mathbf{J}_N[i, j] := \begin{cases} 1, & \text{if } (i - j = 1 \text{ and } i \text{ is even}) \text{ or } (j - i = 1 \text{ and } j \text{ is even}) \\ 0, & \text{else} \end{cases}$$

**Definition 2.28.** ([4]) We denote by  $\sim_c$  the congruence relation of matrices, i.e.

$$\mathbf{A} \sim_c \mathbf{B} \iff \exists \mathbf{Q}, \det(\mathbf{Q}) \neq 0 : \mathbf{B} = \mathbf{Q} \mathbf{A} \mathbf{Q}^\top.$$

We recall the Theorem 1 of [4].

**Theorem 2.29.** *Let  $\mathbf{A} \in M_{N \times N}(\mathbb{F}_2)$  be symmetric with rank  $k$ . Then we have the following.*

- (i) *If every diagonal element of  $\mathbf{A}$  is 0, then  $\mathbf{A} \sim_c \mathbf{J}_k$  and hence  $k$  is even.*

**Remark 2.30.** *In the above, if  $k \leq n$ , when we say  $\mathbf{A} \sim_c \mathbf{J}_k$ , we mean*

$$\mathbf{A} \sim_c \begin{pmatrix} \mathbf{J}_k & 0 \\ 0 & 0_{N-k} \end{pmatrix} \in M_{N \times N}(\mathbb{F}_2).$$

Our  $\Gamma_{\mathcal{A}}$  matrices fit exactly the description in the theorem above, and regardless of the equivalence class representative that [1] found, we know that this equivalence representative class using  $\mathbf{J}_k$  is just as valid (in the sense that both of these representatives are in the same equivalence class). All we need to do now is to figure out what restrictions on  $k$  lead to an MCP equivalence class representative. Therefore, we can only look to the ranks of  $\Gamma_{\mathcal{A}}$  matrices to characterize the set  $\mathcal{A}$ . It follows immediately:

**Theorem 2.31.** (Characterizing  $\mathcal{A}$  via Matrix Rank) *Let  $\mathcal{A}$  be a MCP for a given Lie algebra  $\mathfrak{g}$  and let  $\mathcal{A}'$  be a set of bracket-independent Pauli strings. We have that:*

$$\mathcal{A}' \text{ is MCP for } \mathfrak{g} \iff (\text{rank}(\Gamma_{\mathcal{A}}) = \text{rank}(\Gamma_{\mathcal{A}'})) \wedge (|\mathcal{A}| = |\mathcal{A}'|).$$

*Proof.* The proof uses the ideas introduced above and Lemma 1 in [4]  $\square$

**Corollary 2.32.** *Let  $\mathcal{A}$  be a MCP for a given Lie algebra  $\mathfrak{g}$  and let  $\mathcal{A}'$  be a set of bracket-independent Pauli strings. We have that:*

$$(\text{rank}(\Gamma_{\mathcal{A}}) = \text{rank}(\Gamma_{\mathcal{A}'})) \implies \mathcal{A}' \text{ is a CP for } \mathfrak{g}.$$

### 3 Outlook on Applications

#### 3.1 ADAPT-VQE

The ADAPT-VQE algorithm [2] was introduced as an alternative to VQE. It has showed to achieve a significant reduction in redundant terms within the ansatz. This results in more compact and efficient quantum circuits for molecular simulations. The general framework of ADAPT-VQE is as follows: Given a set of admissible Hermitian generators, denoted as  $\mathbb{P}$ . We define a pool of parametrized unitary operators as  $\mathbb{S} = \{\mathbf{U}(\theta) = \exp(i\theta P) : \theta \in [-\pi, \pi), P \in \mathbb{P}\}$ , where  $P_k$ ,  $k \in [|\mathbb{P}|]$  are the Pauli strings and let  $\mathbf{H} \in \mathbb{R}^{2^N \times 2^N}$  be the Hamiltonian matrix, with  $N$  being the number of qubits:

1. Start with an initial state  $|\Psi_0\rangle$ . A Hartree-Fock state is commonly used as the initial state. (on the quantum hardware, the qubits are booted to the initial state.)
2. Define the pool of unitary operators that will be used to construct the ansatz.
3. At iteration  $k$ , identify the Hermitian operator  $P_j^{(k)} \in \mathbb{P}, j \in [|\mathbb{P}|]$ , such that the action of  $\exp(i\theta_k P_j^{(k)}), \theta_k \in [-\pi, \pi)$  on the previous ansatz (at iteration  $k - 1$ ) is likely to result in the largest decrease in energy. This can be determined by evaluating the following gradient of the energy with respect to  $\theta_k$ : ( This step is done on the quantum Hardware)

$$P^{(k)} = \operatorname{argmax}_{P_j \in \mathbb{P}} \left| \frac{\partial}{\partial \theta} \langle \Psi^{(k-1)} | \exp(i\theta P_j) \mathbf{H} \exp(-i\theta P_j) | \Psi^{(k-1)} \rangle \Big|_{\theta=0} \right|. \quad (10)$$

4. Exit the iteration process if the stopping criteria is met (convergence). Otherwise, append the action  $\exp(i\theta_k P^{(k)})$  to the previous ansatz at iteration  $k - 1$ ,

$$|\Psi^{(k)}\rangle = \exp(-i\theta_k P^{(k)}) |\Psi^{(k-1)}\rangle. \quad (11)$$

5. Optimize all parameters  $\theta_1, \theta_2, \dots, \theta_k$  in the new updated ansatz  $|\Psi^{(k)}\rangle$  by solving the following optimization problem

$$\boldsymbol{\theta}^* = (\theta_1^*, \theta_2^*, \dots, \theta_k^*) = \operatorname{argmin}_{\theta_1, \theta_2, \dots, \theta_k} \langle \Psi^{(0)} | \prod_{j=1}^k \exp(i\theta_j P^{(j)}) \mathbf{H} \prod_{j=k}^1 \exp(-i\theta_j P^{(j)}) | \Psi^{(0)} \rangle. \quad (12)$$

6. Define the new ansatz with the new parameters  $\boldsymbol{\theta}^*$ , such that

$$|\Psi^{(k)}\rangle = \prod_{j=1}^k \exp(-i\theta_j^* P^{(j)}) |\Psi^{(0)}\rangle. \quad (13)$$

There are many types of operator pools that can be used to construct the ADAPT-VQE ansatz such as Qubit-Excitation-Based (QEB) pool [10], Qubit hardware-efficient pool [5] and Minimal Complete pool (MCP) also known as Minimal hardware efficient pool first appeared in [9].

#### 3.2 Symmetries and properties of operator pools:

We introduce in the following different properties and symmetries imposed on the operator pools in order to simulate molecular Hamiltonians:

- **Odd Pauli strings:** The construction of a real ansatz imposes a constraint on its generators  $\mathcal{A} = \{P_i\}_{i \in [|\mathcal{A}|]}$ . To ensure the ansatz maps real states to real states, each Pauli string  $P_i$  in the pool must contain an odd number of Pauli  $Y$  matrices. For example, the four-qubit Pauli string  $P = X_0 Y_1 X_2 X_3$  satisfies this condition because it contains one  $Y$ . We now identify the algebraic structure generated by this subset of Pauli strings.

**Proposition 3.1.** *Given a Pauli string  $\alpha$ , the number of  $Y$  terms in the Pauli string is given by*

$$e_p : \mathbb{F}_2^{2N} \longrightarrow \mathbb{N}$$

$$v \longmapsto e_p(v),$$

such that for  $\alpha \in i\mathcal{P}_N^*$ ,

$$e_p(\phi(\alpha)) := (v_X^\alpha)^\top v_Z^\alpha,$$

where  $\phi(\alpha) = (v_X^\alpha, v_Z^\alpha)$ , as defined in 2.9.

*Proof.*  $(v_X^\alpha)^\top v_Z^\alpha$  is a sum over all tensor product slots, each individual summand can only be a 1 if both an  $X$  and  $Z$  term appears in the same slot, which is exactly the condition for a  $Y$  term to be created.  $\square$

**Proposition 3.2.** *If  $\alpha, \beta$  are two odd Pauli strings that anti-commute, then  $[\alpha, \beta]$  and  $\alpha \circ \beta$  are also both odd Pauli strings.*

*Proof.* Let  $\phi(\alpha) = (v_X^\alpha, v_Z^\alpha)$ , and  $\phi(\beta) = (v_X^\beta, v_Z^\beta)$ , thus

$$e_p(\phi(\alpha) + \phi(\beta)) = (v_X^\alpha + v_X^\beta)^\top (v_Z^\alpha + v_Z^\beta) = (v_X^\alpha)^\top v_Z^\alpha + (v_X^\alpha)^\top v_Z^\beta + (v_X^\beta)^\top v_Z^\alpha + (v_X^\beta)^\top v_Z^\beta$$

$$= 1 + \lambda + \mu + 1 = \lambda + \mu = 1,$$

where arithmetic operations in the above are all  $(\text{mod } 2)$ . We use the fact that  $(v_X^\alpha)^\top v_Z^\alpha$  gives us the number of  $Y$  terms in  $\alpha$ , and similarly for  $(v_X^\beta)^\top v_Z^\beta$  in  $\beta$ . Then,  $\lambda$  and  $\mu$  are exactly given by  $(v_X^\beta)^\top v_Z^\alpha$  and  $(v_X^\alpha)^\top v_Z^\beta$ , respectively. Since  $\alpha$  and  $\beta$  anti-commute, according to 2.11,  $\lambda + \mu$  is equal to 1, we can conclude the proof.  $\square$

It follows:

**Proposition 3.3.** *Let  $i\mathcal{P}_N^\mathcal{O}$  be the subset of Odd Pauli strings in  $i\mathcal{P}_N$ , then the set*

$$i\mathcal{P}_N^\mathcal{O} \cup \{0\},$$

*is closed under the commutator (up to a scalar).*

**Proposition 3.4.** *The set  $\text{span}_\mathbb{R}(i\mathcal{P}_N^\mathcal{O})$  is exactly the Lie algebra  $\mathfrak{so}(2^N, \mathbb{R})$ .*

*Proof.* Recall that  $\mathfrak{su}(2^N) = \text{span}_\mathbb{R}(i\mathcal{P}_N^*)$ , i.e.,  $i\mathcal{P}_N^*$  is a real (Hamel) basis for the skew-Hermitian matrices of vanishing trace. Now, if we consider  $i\mathcal{P}_N^\mathcal{O}$ , then  $\text{span}_\mathbb{R}(i\mathcal{P}_N^\mathcal{O})$  is the set of all skew-symmetric (the skew-Hermitian property is  $A^\dagger = -A$ , but since we have real matrices now, we have  $A^\top = -A$ , hence, skew-symmetric) real matrices of vanishing trace. Note that skew-symmetric matrices automatically have vanishing trace. Now, note that the set of skew-symmetric matrices (equipped with the commutator bracket) is exactly the Lie algebra  $\mathfrak{so}(2^N, \mathbb{R})$ .  $\square$

**Proposition 3.5.** *The cardinality of the set  $i\mathcal{P}_N^\mathcal{O}$  is  $|i\mathcal{P}_N^\mathcal{O}| = \frac{1}{2}2^N(2^N - 1)$ .*

*Proof.* Given  $N$ -qubit system, we will try to count the cardinality of  $i\mathcal{P}_N^\mathcal{O}$ , i.e., the subset of odd strings from  $i\mathcal{P}_N$ . We will proceed following a combinatorial approach: First, consider  $N$  empty slots arranged in a row as:

$$(\circ \quad \circ \quad \circ \quad \cdots \quad \circ)$$

We first pick the slots to be filled with  $Y$  terms. For example, if we want exactly 5  $Y$  slots in a row of  $N$  total slots, we must choose 5 positions. The number of ways to choose these positions is  $\binom{N}{5}$  one such choice might look like this ( $\circ$  represents empty slots)

$$(Y \quad Y \quad Y \quad \circ \quad Y \quad \circ \quad \dots \quad Y \quad \circ).$$

For each  $\binom{N}{5}$  ways, we have  $N - 5$  empty slots remaining. Each of these empty slots can be filled with any of the other Pauli operators:  $\{I, X, Z\}$ . Since there are  $N - 5$  slots and 3 choices for each, the number of ways to fill the remaining slots is  $3^{N-5}$ . In this case,  $\binom{N}{5} \cdot 3^{N-5}$  is the number of odd Paulis having exactly 5  $Y$  terms.

Now, if we sum these quantities over all of the odd numbers  $2p + 1$  from 1 to  $N$ , we obtain

$$|i\mathcal{P}_N^{\mathcal{O}}| = \sum_{p=0}^{\frac{1}{2}(N-2)} \binom{N}{2p+1} \cdot 3^{N-(2p+1)}$$

Note that we assume  $N$  is even, therefore the last odd number we sum over is  $N - 1$ , hence why our upper bound in the sum is  $\frac{1}{2}(N - 2)$ . Equivalently, we can write this as

$$|i\mathcal{P}_N^{\mathcal{O}}| = \sum_{p=1, p \text{ odd}}^{N-1} \binom{N}{p} \cdot 3^{N-p}.$$

This sum can be simplified further. We recall some binomial relations:

$$(\alpha + \beta)^N = \sum_{p=0}^N \binom{N}{p} \alpha^p \beta^{N-p}, \text{ and } (\alpha - \beta)^N = \sum_{p=0}^N \binom{N}{p} (-1)^{N-p} \alpha^p \beta^{N-p}.$$

It follows:

$$(\alpha + \beta)^N - (\alpha - \beta)^N = \sum_{p=0}^N \binom{N}{p} (1 - (-1)^{N-p}) \alpha^p \beta^{N-p}$$

We have that  $1 - (-1)^{N-p}$  is 0 when  $p$  is even. Hence,

$$(\alpha + \beta)^N - (\alpha - \beta)^N = 2 \cdot \sum_{p=0, p \text{ odd}}^N \binom{N}{p} \alpha^p \beta^{N-p}.$$

Now, if we set  $\alpha = 1$  and  $\beta = 3$ , we obtain

$$|i\mathcal{P}_N^{\mathcal{O}}| = \frac{1}{2}((1 + 3)^N - (1 - 3)^N) = \frac{1}{2}(4^N - 2^N) = \frac{1}{2}(2^{2N} - 2^N) = \frac{1}{2}2^N(2^N - 1)$$

This corresponds to the real dimension of the Lie algebra  $\mathfrak{so}(2^N)$ . □

Now we move to the next property of Pauli strings in our desired operator pool. First, we can define a state where the single-particle orbitals are ordered by spin projection. For spin- $\frac{1}{2}$  particles, we use the notation  $\mu$  for spin-up ( $m_s = +\frac{1}{2}$ ) and  $\nu$  for spin-down ( $m_s = -\frac{1}{2}$ ). A state can be expressed as:

$$|\psi\rangle = |\mu\nu\mu\nu\dots\rangle.$$

- **EvenFlip:** The even flip property is satisfied if a Pauli string contains an even number of spin-flipping operations (Pauli X or Y) for each spin orbital  $\mu$  and  $\nu$ , independently. One can translate the even flip property into an equivalent condition on the corresponding vectors in  $\mathbb{F}_2^{2N}$

**Definition 3.6.** Let  $N$  be the number of spin-orbital pairs. Let  $\phi : i\mathcal{P}_N^* \rightarrow \mathbb{F}_2^{2N}$  be the mapping from a Pauli string  $\alpha \in i\mathcal{P}_N^*$  to its  $2N$ -dimensional vector representation such that  $v = \phi(\alpha)$ . Given a set  $\mathcal{A}$  of Pauli strings, we define the following matrices:  $|\mathcal{A}| \times 2N$  matrices  $E_\mu$  and  $E_\nu$  project onto the odd-indexed ( $\mu$ ) and even-indexed ( $\nu$ ) spin-orbital components, respectively.

$$E_\mu := \begin{pmatrix} e_1^\top \\ e_3^\top \\ \vdots \\ e_{2N-1}^\top \end{pmatrix}, \quad E_\nu := \begin{pmatrix} e_2^\top \\ e_4^\top \\ \vdots \\ e_{2N}^\top \end{pmatrix}$$

(Here,  $e_i$  is the  $i$ -th standard basis vector of  $\mathbb{F}_2^{2N}$ ). We define also the  $2N$ -dimensional vector  $b_Z$  as:

$$b_Z := \begin{pmatrix} 0_N \\ 1_N \end{pmatrix}.$$

Let  $\Lambda$  be a predefined  $(2N \times 2N)$  matrix (as given in 2.9). We define the parity functions  $e_f^\mu, e_f^\nu : \mathbb{F}_2^{2N} \rightarrow \mathbb{Z}$  as:

$$e_f^\mu(v) := (E_\mu(v) + b_Z)^\top \Lambda (E_\mu(v))$$

$$e_f^\nu(v) := (E_\nu(v) + b_Z)^\top \Lambda (E_\nu(v))$$

These functions are intended to count properties (like the number of X and Y terms) related to the  $\alpha$  and  $\beta$  spin-orbitals.

**Definition 3.7.** (Even Flip Property) A Pauli string  $\alpha \in i\mathcal{P}_N^*$ , with vector representation  $v = \phi(\alpha) \in \mathbb{F}_2^{2N}$ , is defined to satisfy the even flip property if both of its parity-check functions evaluate to an even number.

$$e_f^\mu(v) \equiv 0 \pmod{2} \quad \text{and} \quad e_f^\nu(v) \equiv 0 \pmod{2}$$

**Proposition 3.8.** The set of Pauli strings that preserve the even flip property is closed under the commutator (up to a scalar).

*Proof.* We need to show that if two Pauli strings  $\alpha, \beta \in i\mathcal{P}_N^*$  preserve the even flip, then  $[\alpha, \beta]$  and  $\alpha\beta$  also preserve the even flip. Let  $v_\alpha = \phi(\alpha)$  and  $v_\beta = \phi(\beta)$ . Demonstrating that  $\alpha\beta$  also preserve the even flip is equivalent to showing that  $v_\alpha + v_\beta$  preserve the even flip. We proceed as follows:

$$\begin{aligned} e_f^\mu(v_1 + v_2) &= (E_\mu(v_1) + E_\mu(v_2) + b_Z)^\top \Lambda (E_\mu(v_1) + E_\mu(v_2)) \pmod{2} \\ &= (E_\mu(v_1) + b_Z)^\top \Lambda E_\mu(v_2) + E_\mu(v_2)^\top \Lambda E_\mu(v_1) + E_\mu(v_2)^\top \Lambda E_\mu(v_2) \pmod{2} \\ &= E_\mu(v_2)^\top \Lambda E_\mu(v_2) + b_Z^\top \Lambda E_\mu(v_2) + 2E_\mu(v_2)^\top \Lambda E_\mu(v_1) \pmod{2} \\ &= 0 \pmod{2}, \end{aligned} \tag{14}$$

where  $E_\mu(v_2)^\top \Lambda E_\mu(v_2)$  is the number of Y terms acting on  $\mu$  which is even and  $b_Z^\top \Lambda E_\mu(v_2)$  is the number of X terms acting on  $\mu$  which is also even. Using similar arguments, we can show that  $e_f^\nu(v_1 + v_2) = 0 \pmod{2}$ .  $\square$

We conclude that the set of operators satisfying both the even flip and odd string properties generates a subalgebra of  $\mathfrak{so}(2^n)$ .

In order to improve algorithmic convergence, the initial set of operators (or starters) used to construct the complete operator pool is restricted by imposing the following additional symmetries and properties on the Pauli strings:

- **Particle number conservation:** A Pauli string  $\alpha$  conserves the particle number if the number of  $X$  or  $Y$  terms in the first half of the string is equal to the number of  $X$  or  $Y$  terms in the second half of the string. For instance, consider a four-qubit system where a two-particles state is defined as  $|1100\rangle$ . Applying the Pauli operator  $XIII$  to this state transforms it into  $|0100\rangle$ , which corresponds to a state with only one particle. This operation violates particle number conservation, as it changes the particle count.
- **Single and double excitations:** Only operators corresponding to single and double excitations are included. This is a physical constraint derived from the molecular Hamiltonian, which typically contains only one and two-body interaction terms. Any operator that would generate triple, quadruple, or higher-order excitations is excluded. For example, a Pauli string that transforms the state  $|11110000\rangle$  (four particles) to  $|00001111\rangle$  (four particles in different orbitals) would not be allowed, as this represents a quadruple excitation.

We note that Point group and spin symmetries are also taken into account, as considered in [3].

## 4 Existing methods on pool completeness:

**Full Lie Algebra check:** the work of [9], demonstrates that the completeness of a Pauli string pool,  $\mathcal{A} = \{P_i\}_{i \in [|\mathcal{A}|]}$ , can be verified by analyzing the rank of a matrix  $\mathbf{M} \in \mathbb{R}^{|\mathcal{A}| \times |\mathcal{A}|}$ . Given an arbitrary state  $|\Psi\rangle$ , this matrix is defined as  $\mathbf{M} \in \mathbb{R}^{|\mathcal{A}| \times |\mathcal{A}|}$  with entries  $\mathbf{M}[i, j] = \langle \Psi | P_i^\top P_j | \Psi \rangle$ . The pool is said to be complete if its rank satisfies  $\text{rank}(\mathbf{M}) \geq 2^N - 1$ . This rank condition signifies that the set of states  $\{P_i|\Psi\rangle\}_{i \in [|\mathcal{A}|]}$  forms a complete basis, and consequently, any state in the Hilbert space can be expressed as a linear combination of these basis elements. In practice, a "generate-and-test" approach is performed: random pools are generated, and their rank is evaluated afterward. The complexity of this rank evaluation is polynomial in  $N$ , assuming the pool size  $|\mathcal{A}|$  scales linearly with  $N$ . However, the primary computational bottleneck is the construction of  $\mathbf{M}$ , as the naive evaluation of its entries scales exponentially.

**Product group size+inseparability criteria:** According to theorems of completeness in [7], a minimal complete pool comprised of odd Pauli strings must contain  $2N - 2$  elements. This pool generates a product group (built through all possible products of the operators in the set) of size  $\frac{2^{N-1}(2^{N-1}+1)}{2}$ . The Lie algebra generated by this pool is the subset of all odd Pauli strings within the product group, and its size is  $\frac{2^{N-1}(2^{N-1}-1)}{2}$ . The authors in [7] formulated necessary and sufficient conditions for verifying MCPs in the molecular case, which are outlined as "practical recipe". These steps include:

1. **Check the product group:** Generate the product group from the pool and verify that it coincides with the canonical group from the paper's theorem.
2. **Verify the Inseparability Condition:** Check that the pool's generators cannot be split into two mutually commuting sets.
3. **Full Lie Algebra check (Optional):** Analytically prove completeness by building the Lie algebra and verifying that it spans all odd strings from the group. The authors note

this step is very resource demanding and suggest that satisfying the first two conditions is sufficient for practical purposes.

**Greedy pool construction:** The authors in [6] build upon the completeness theorems proposed in [7]. They introduce an efficient and automated procedure to check the product group size. This method represents each Pauli string in the pool  $\mathcal{A}$  as a  $2N$ -length bitstring. Gaussian elimination is then performed on the resulting  $|\mathcal{A}| \times 2N$  matrix of these bitstrings to find the matrix rank  $K$ , the group size is subsequently determined as  $2^K$ . Following the practical recipe suggested in [7], this approach bypasses the computationally "very resource demanding" step of explicitly constructing and verifying the full Lie algebra, as the first two conditions are considered to be sufficient for practical verification. However, this does not always guarantee the completeness.

## 5 DATA

### 5.1 Geometries

Table 1: Geometries (in Å) of the molecular systems studied present in the paper.

| System           |     | x  | y       | z        |
|------------------|-----|----|---------|----------|
| LiH              | Li  | 0. | 0.      | 0.       |
|                  | H   | 0. | 0.      | 1.3      |
| H <sub>2</sub> O | O   | 0. | 0.      | 0.1173   |
|                  | H   | 0. | 0.7572  | -0.4692  |
|                  | H   | 0. | -0.7572 | -0.4692  |
| H <sub>n</sub>   | H   | 0. | 0.      | 0.0      |
|                  | H   | 0. | 0.      | d        |
|                  | ... |    |         |          |
|                  | H   | 0. | 0       | d(n - 1) |

where for H<sub>6</sub> molecule we have  $d = 3$  and for H<sub>8</sub> molecule  $d = 0.8$ .

## References

- [1] Gerard Aguilar, Simon Cichy, Jens Eisert, and Lennart Bittel. Full classification of pauli lie algebras. *ArXiv:2408.00081* <https://arxiv.org/abs/2408.00081>, 2024.
- [2] Harper R. Grimsley, Sophia E. Economou, Edwin Barnes, and Nicholas J. Mayhall. An adaptive variational algorithm for exact molecular simulations on a quantum computer. *Nature Communications*, 10(1), July 2019.
- [3] Mohammad Haidar, Olivier Adjoua, Siwar Badreddine, Alberto Peruzzo, and Jean-Philip Piquemal. Non-iterative disentangled unitary coupled-cluster based on lie-algebraic structure. *Quantum Science and Technology*, 10(2):025031, February 2025.
- [4] YONG-HYUK KIM and Keomkyo Seo. Two congruence classes for symmetric binary matrices over f2. *WSEAS Transactions on Mathematics*, 7, 01 2008.
- [5] Ilya G. Ryabinkin, Tzu-Ching Yen, Scott N. Genin, and Artur F. Izmaylov. Qubit coupled cluster method: A systematic approach to quantum chemistry on a quantum computer. *Journal of Chemical Theory and Computation*, 14(12):6317–6326, 2018. PMID: 30427679.
- [6] Mariia D. Sapova and Aleksey K. Fedorov. Variational quantum eigensolver techniques for simulating carbon monoxide oxidation. *Communications Physics*, 5(1), August 2022.

- [7] V. O. Shkolnikov, Nicholas J. Mayhall, Sophia E. Economou, and Edwin Barnes. Avoiding symmetry roadblocks and minimizing the measurement overhead of adaptive variational quantum eigensolvers. *Quantum*, 7:1040, June 2023.
- [8] Isaac D. Smith, Maxime Cautrès, David T. Stephen, and Hendrik Poulsen Nautrup. Optimally generating  $\mathfrak{su}(2^N)$  using pauli strings. *Physical Review Letters*, 134(20), May 2025.
- [9] Ho Lun Tang, V.O. Shkolnikov, George S. Barron, Harper R. Grimsley, Nicholas J. Mayhall, Edwin Barnes, and Sophia E. Economou. Qubit-adapt-vqe: An adaptive algorithm for constructing hardware-efficient ansätze on a quantum processor. *PRX Quantum*, 2(2), April 2021.
- [10] Yordan S. Yordanov, V. Armaos, Crispin H. W. Barnes, and David R. M. Arvidsson-Shukur. Qubit-excitation-based adaptive variational quantum eigensolver. *Communications Physics*, 4(1), October 2021.
